# Supplementary material for: T\^atonnement in Homothetic Fisher Markets
Source: arXiv:2306.04890 source file (2025-02-28)
Supplement: Supplementary file 1 [file proofs_sec3.tex]

\equivoptim*

\begin{proof}[\Cref{equiv-optim}]
The Lagrangian associated with $\max_{\allocation[\buyer]: \allocation[\buyer] \cdot \price \leq \budget[\buyer]} \budget[\buyer] \log (\util[\buyer](\allocation[\buyer]))$ is given by:
\begin{align*}
    L(\allocation[
    \buyer], \lambda, \bm{\mu}) = \budget[\buyer] \log( \util[\buyer] (\allocation[\buyer])) + \lambda \left(  \budget[\buyer] - \allocation[\buyer] \cdot \price \right) + \bm{\mu}^T \allocation[\buyer] \enspace ,
\end{align*}

\noindent
where $\lambda \in \R_+$ and $\bm \mu \in \R^\numgoods_+$ are slack variables.

Let $(\allocation[\buyer]^*, \lambda^*, \bm \mu^*)$ be an optimal solution to the Lagrangian.
From the KKT stationarity condition for this Lagrangian  \cite{kuhn1951kkt}, it holds that, for all $\good \in \goods$,
\begin{align*}
    \frac{\budget[\buyer]}{\util[\buyer] (\allocation[\buyer]^*)} \left[ \frac{\partial \util[\buyer]}{\partial \allocation[\buyer][\good]} \right]_{\allocation[\buyer] = \allocation[\buyer]^*} - \lambda^* \price[\good] + \mu_{\good}^* \doteq 0 \\
    \frac{\budget[\buyer]}{\util[\buyer] (\allocation[\buyer]^*)} \left[ \frac{\partial \util[\buyer]}{\partial \allocation[\buyer][\good]} \right]_{\allocation[\buyer] = \allocation[\buyer]^*} \allocation[\buyer][\good]^* - \lambda^* \price[\good] \allocation[\buyer][\good]^* + \mu_{\good}^* \allocation[\buyer][\good]^* = 0 \\
    \frac{\budget[\buyer]}{\util[\buyer] (\allocation[\buyer]^*)} \left[ \frac{\partial \util[\buyer]}{\partial \allocation[\buyer][\good]} \right]_{\allocation[\buyer] = \allocation[\buyer]^*} \allocation[\buyer][\good]^* - \lambda^* \price[\good] \allocation[\buyer][\good]^* = 0
    \enspace .
\end{align*}
\noindent
The penultimate line is obtained by multiplying both sides by $\allocation[\buyer][\good]^*$, and the last line, by the KKT complementarity condition, namely $\mu_{\good}^* \allocation[\buyer][\good]^* = 0$.

Summing up across all $\good \in \goods$ on both sides yields:
\begin{align*}
    \frac{\budget[\buyer]}{\util[\buyer](\allocation[\buyer]^*)} \sum_{\good \in \goods}\left[\frac{\partial \util[\buyer]}{\partial \allocation[\buyer][\good]}\right]_{\allocation[\buyer] = \allocation[\buyer]^*}\allocation[\buyer][\good]^* - \lambda^* \sum_{\good \in \goods} \price[\good] \allocation[\buyer][\good]^*  = 0\\
    \frac{\budget[\buyer]}{\util[\buyer](\allocation[\buyer]^*)}\util[\buyer](\allocation[\buyer]^*) - \lambda^* \sum_{\good \in \goods} \price[\good] \allocation[\buyer][\good]^*  = 0\\
    \budget[\buyer] -\lambda^* \budget[\buyer]  = 0\\
    \lambda^* = 1 \enspace ,
\end{align*}

\noindent
‚where the second line is obtained from Euler's theorem for homogeneous functions \cite{lewis1969homogeneous}, and the last line, from the KKT complementarity condition again, namely $\lambda^* \left(\sum_{\good \in \goods} \budget[\buyer] - \price[\good] \allocation[\buyer][\good]^* \right) = 0$.

Hence, plugging $\lambda^* = 1$
back into the Lagrangian restricted to $\R^\numgoods_+$, we get:
\begin{align*}
    \max_{\allocation[\buyer] \in \R^\numgoods_+: \allocation[\buyer] \cdot \price \leq \budget[\buyer]} \budget[\buyer] \log (\util[\buyer] (\allocation[\buyer])) &= \max_{\allocation[\buyer] \in \R^\numgoods_+} \budget[\buyer] \log( \util[\buyer] (\allocation[\buyer])) + \lambda^* \left( \budget[\buyer] -   \allocation[\buyer] \cdot \price \right)\\
    &= \max_{\allocation[\buyer] \in \R^\numgoods_+} \budget[\buyer] \log(\util[\buyer] (\allocation[\buyer])) + \budget[\buyer] - \allocation[\buyer] \cdot \price  \enspace .
\end{align*}
\end{proof}

Recall that the dual proposed by \citeauthor{cole2019balancing} \cite{cole2019balancing} is given by: 
\begin{align*}
    \min_{\price \in \R^\numgoods} \sum_{\good \in \goods} \price[\good] + \sum_{\buyer \in \buyers} \budget[\buyer] \log(\util[\buyer](\allocation[\buyer]))
\end{align*}

This dual's optimal differs from the optimal value of the Eisenberg-Gale program by a constant factor (of $\sum_{\buyer \in \buyers} \budget[\buyer]$) as shown by the following example:

\begin{example}\label{dual-diff-cole}
Consider a linear Fisher market with only one good and one buyer with a utility of $1$ for the good and a budget of $1$ as well.
The equilibrium of this market is given by $\allocation[1][1]^* = 1, \price[1]^* = 1$. 
The primal of the Eisenberg-Gale program thus evaluates to $\budget[1]\log(\allocation[1][1]^*) = (1) \log(1) = 0$, while the dual given by \citeauthor{cole2019balancing} evaluates to $1 \log(1) + 1 = 1$.
Hence, the optimal primal value is not equal to the optimal dual value of the dual given by \citeauthor{cole2019balancing}, so this dual is not exactly the dual of the Eisenberg-Gale program.
\end{example}
